# Supplementary material for: On Causally Disentangled State Representation Learning for Reinforcement Learning based Recommender Systems
Source: arXiv:2407.13091 source file (2024-07-18)
Supplement: Supplementary file 1 [file appendix.tex]

\section{A.}
